# Supplementary material for: Deep Generative Models of Music Expectation
Source: arXiv:2310.03500 source file (2023-10-05)
Supplement: Supplementary file 1 [file appendix_a.tex]

\section{Experiment Details}
